# Supplementary material for: Theory of the tertiary instability and the Dimits shift from reduced drift-wave models
Source: arXiv:1910.05227 ancillary file (2019-12-11)
Supplement: Supplementary file 1 [file Supplemental_Material.pdf]

# Theory of the tertiary instability and the Dimits shift from reduced drift-wave models: Supplemental Material

Hongxuan Zhu,[1,2] Yao Zhou,[1] and I. Y. Dodin[1,2]

[1] *Princeton Plasma Physics Laboratory, Princeton, NJ 08543*

[2] *Department of Astrophysical Sciences, Princeton University, Princeton, NJ 08544*

Here, we show that our general approach to understanding the tertiary instability (TI) extends beyond the Hasegawa–Wakatani model assumed in the main text. Specifically, we consider electrostatic ion-temperature-gradient (ITG) turbulence and explore the corresponding tertiary modes both numerically and analytically.

First, we perform gyrokinetic simulations using the code GS2 [1] to check for the localization of the tertiary modes. For simplicity, the simulations are done in slab geometry with zero magnetic shear. The simulation domain is a three-dimensional periodic box with lengths $L_x = L_y = 10\pi\rho_{\rm i}$ and $L_z = 20\pi a$. Here, $\rho_{\rm i}$ is the ion gyroradius at thermal speed, and $a$ is a reference length. Ions have finite gradients of the temperature and density, with the corresponding scale lengths $L_T = 0.5a$ and $L_n = 2.5a$. The electron temperature is equal to the ion temperature, and the electron response is assumed adiabatic except with respect to the zonal mode, as usual [3]. Ion–ion collisions are included with the rate $\nu_{\rm ii} = 0.05 v_{\rm i}/a$, where $v_{\rm i}$ is the ion thermal velocity [4, 5]. The simulation results are shown in Fig. 1, which shows that ITG modes tend to localize near the extrema of the zonal-flow (ZF) velocity $U$. Therefore, the general approach used in the main text naturally extends to these modes.

A detailed study of the localized ITG modes within the gyrokinetic formulation is beyond the scope of this note. However, an intuitive understanding can be obtained by

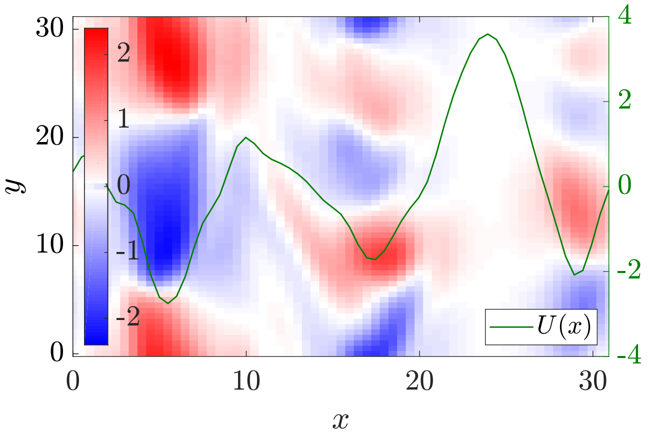


FIG. 1. GS2 simulation results showing the electrostatic potential (color) and the ZF velocity $U$ (green curve) at $z = 0$. ITG modes are localized near the extrema of $U$.

revisiting the two-dimensional gyrofluid model used in Ref. [2]. The model equations are

$$\partial_t n + [\phi, n] + [\tau\nabla^2\phi, T]/2 = 0, \quad \partial_t T + [\phi, T] = 0, \quad (1)$$

where $[f,g] \doteq \hat{\boldsymbol{z}} \times \nabla f \cdot \nabla g$ for any scalar $f$ and $g$, $\tau = T_{\rm i0}/T_{\rm e0}$, $\phi$ is the perturbation of the gyroaveraged electrostatic potential, $T$ is the perturbation of the ion-guiding-center perpendicular temperature, and $n \doteq (1-\tau\nabla^2)(\phi - \langle\phi\rangle) - \nabla^2(\phi + \tau T/2)$ is the perturbation of the ion-guiding-center density. To study the TI, let us consider $\phi = \phi_0(x) + \tilde{\phi}(x)\mathrm{e}^{\mathrm{i}(p_y y - \omega t)}$ and $T = T_0(x) + \tilde{T}(x)\mathrm{e}^{\mathrm{i}(p_y y-\omega t)}$, where $\phi_0$ and $T_0$ are zonal perturbations; in particular, $T_0$ plays the same role as $N$ in the main text. Then, $n_0 = -\phi_0'' - \tau T_0''/2$ and $\tilde{n} = (1 + \tau\hat{p}^2 + \hat{p}^2)\tilde{\phi} + \tau\hat{p}^2\tilde{T}/2$, where $\hat{p}^2 \doteq -\nabla^2$. Let us define $U(x) \doteq \phi_0'$, $\bar{\omega}(x) \doteq \omega - p_y U$, and assume that $\eta \doteq T_0'$ is a positive constant. Then, Eqs. (1) lead to the eigenmode equation $\omega\tilde{n} = \hat{H}\tilde{n}$ with

$$\hat{H} = p_y U + p_y \left[U'' + \frac{\tau\eta\hat{p}^2}{2} - \frac{p_y\tau\eta U''}{2\bar{\omega}}\right]\hat{A}^{-1}, \quad (2)$$

where $\hat{A} = 1 + (1+\tau)\hat{p}^2 - p_y\eta\tau\bar{\omega}^{-1}\hat{p}^2/2$. Since we expect the modes to be localized, we assume $U \approx U_0 + \mathcal{C}x^2/2$, where $\mathcal{C} \doteq U''(0)$. Then, we expand the Hamiltonian as $\hat{H} \approx \mathcal{H} + \lambda_p\,\hat{p}_x^2 + \lambda_x\,x^2$, where

$$\mathcal{H} = p_y U_0 + \frac{p_y^3\tau\eta}{2A_0} - \frac{p_y^2\tau\eta\mathcal{C}}{2\bar{\omega}_0 A_0}, \quad \bar{\omega}_0 \doteq \omega - p_y U_0, \quad (3)$$

$$\lambda_p = \frac{p_y\tau\eta}{2A_0} + \frac{p_y^4\tau^2\eta^2}{4\bar{\omega}_0 A_0^2} - \frac{p_y^3\tau^2\eta^2\mathcal{C}}{4\bar{\omega}_0^2 A_0^2}, \quad (4)$$

$$\lambda_x = \frac{p_y\mathcal{C}}{2} + \frac{p_y^7\tau^2\eta^2\mathcal{C}}{8\bar{\omega}_0^2 A_0^2} - \frac{p_y^6\tau^2\eta^2\mathcal{C}^2}{8\bar{\omega}_0^3 A_0^2} - \frac{p_y^3\tau\eta\mathcal{C}^2}{4\bar{\omega}_0^2 A_0}, \quad (5)$$

In deriving these equations, we have used

$$\hat{A} \approx A_0 - \frac{p_y\eta\tau}{2\bar{\omega}_0}\hat{p}_x^2 - \frac{p_y^4\tau\eta\mathcal{C}}{4\bar{\omega}_0^2}x^2, \quad A_0 \doteq 1 - \frac{p_y^3\eta\tau}{2\bar{\omega}_0}. \quad (6)$$

The ordering $p_y \sim \sqrt{q_{\rm Z}} \ll 1$ has also been assumed like in Ref. [2], where $q_{\rm Z}$ is the characteristic wavenumber of $\phi_0$ and $T_0$. Then, the most-unstable eigenmode has the profile $\tilde{n} \propto \mathrm{e}^{-x^2/2\lambda}$ and complex frequency

$$\omega = \mathcal{H} + \lambda_x\lambda, \quad (7)$$

where $\lambda \doteq \sqrt{\lambda_p/\lambda_x}$ and we choose the branch of the square root such that $\mathrm{Re}\,\lambda > 0$.

From this, one can roughly estimate the growth rate and the mode width as follows. Since the term $\lambda_x\lambda$ acts as a *modification* of the growth rate, let us assume temporarily that it can be ignored. Then, $\bar{\omega}_0 \approx -p_y^2\tau\eta\mathcal{C}/2\bar{\omega}_0 A_0$, which leads to $\omega = p_y U_0 \pm \sqrt{-p_y^2\tau\eta\mathcal{C}/2A_0}$. This shows that $\mathrm{Re}\,\omega \approx p_y U_0$, and the mode is unstable where $\eta\mathcal{C} > 0$, in which case one obtains $\gamma \doteq \mathrm{Im}\,\omega \sim p_y\sqrt{\tau\eta\mathcal{C}}$. The characteristic mode width, $\Delta x \doteq \lambda^{1/2}$, can be estimated from the first terms in $\lambda_p$ and $\lambda_x$ as $\Delta x \sim (\tau\eta/\mathcal{C})^{1/4}$. These results are in agreement with the formulas $\Delta x = (2\tau\eta/\mathcal{C})^{1/4}$ and $\gamma \approx 0.55 p_y\sqrt{\tau\eta\mathcal{C}/2}$ presented in Ref. [2] up to order-one coefficients.

The above calculations can be made more quantitative by assuming $\bar{\omega}_0 = \alpha p_y\sqrt{\tau\eta\mathcal{C}}$, where $\alpha$ is a constant to be determined. Let us assume, as in Ref. [2], that the growth rate is maximized at $p_y \approx (\mathcal{C}/2\tau\eta)^{1/4}$. Then, $A_0 = 1 - 1/2\sqrt{2}\alpha$, and

$$\frac{\mathcal{H} - p_y U_0}{\bar{\omega}_0} = \frac{1}{2\sqrt{2}\alpha A_0} - \frac{1}{2\alpha^2 A_0}, \tag{8}$$

$$\lambda_p = \frac{p_y\tau\eta}{2}\left(\frac{1}{A_0} + \frac{1}{2\sqrt{2}\alpha A_0^2} - \frac{1}{2\alpha^2 A_0^2}\right), \tag{9}$$

$$\lambda_x = \frac{p_y\mathcal{C}}{2}\left(1 + \frac{1}{8\alpha^2 A_0^2} - \frac{1}{4\sqrt{2}\alpha^3 A_0^2} - \frac{1}{2\alpha^2 A_0}\right). \tag{10}$$

Then, Eq. (7) becomes an algebraic equation for $\alpha$. The solution of this equation that corresponds to an instability is $\alpha \approx 0.80 + 0.58\mathrm{i}$, so $\gamma \approx 0.58 p_y\sqrt{\tau\eta\mathcal{C}}$. Also note that $(\mathrm{Re}\lambda_x)(\mathrm{Re}\lambda_p) > 0$ at this value of $\alpha$, so the corresponding mode is a trapped mode. Although the growth rate found here is still different from the result in Ref. [2] by an order-one factor, this calculation shows that our approach accurately captures basic physics of the TI and also reveals details of the mode structure.

Note that in the gyrofluid model considered here, the TI is driven by the zonal perturbation of the ion perpendicular temperature $T_0$. Tertiary modes become stable if only the flow $U = \phi_0'$ is present. (This is mentioned in Ref. [2] and is also seen from the estimate that $\gamma \propto \sqrt{T_0'\phi_0'''}$.) To verify this, we numerically studied $\gamma$ for the ZF profile

$$\phi_0 = q_{\mathrm{Z}}^{-1} u \cos q_{\mathrm{Z}} x, \quad T_0 = -q_{\mathrm{Z}}^{-1}\eta \sin q_{\mathrm{Z}} x. \tag{11}$$

The same slab geometry is assumed as in Fig. 1. We calculated $\gamma$ of the fastest mode from GS2 simulations for various $u$ and $\eta$ such that $u\eta \geq 0$ (Fig. 2). It is seen that at zero $T_0$ ($\eta = 0$), $\gamma$ decreases with $u$. This is consistent with our claim in the main text that the TI is *not* a Kelvin–Helmholtz instability. But if $\eta$ increases with $u$, then $\gamma$ can increase with $u$ at large $u$, which is consistent with results of Ref. [2]. In toroidal geometry, a stationary ZF is uniquely determined as the Rosenbluth–Hinton residual state [6]. Therefore, it is reasonable to expect that $\eta$ generally increases with $u$, as assumed in Ref. [2]. Nevertheless, it is instructive to note that while $T_0$ has a destabilizing effect on tertiary modes, $\phi_0$ has a stabilizing effect on them.

In conclusion, our results elucidate the findings from Ref. [2] by placing the TI theory in a broader context and further demonstrated that the TI is not a Kelvin–Helmholtz instability.

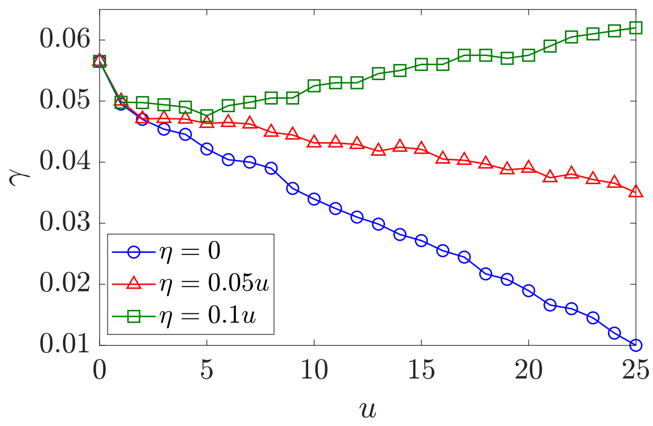


FIG. 2. The fastest tertiary-mode growth rate $\gamma$ from GS2 simulations for the ZF profile (11) with $q_{\mathrm{Z}} = 0.2$ as a function of $u$ for various $\eta$. Here, $\gamma$ is measured in units $v_{\mathrm{i}}/a$, $q_{\mathrm{Z}}$ is measured in units $\rho_{\mathrm{i}}^{-1}$, and $u$ is measured in units $v_{\mathrm{i}}\rho_{\mathrm{i}}/a$. Simulation parameters are the same as in Fig. 1, except $\nu_{\mathrm{ii}} = 10^{-3}v_{\mathrm{i}}/a$ is chosen to avoid heavy damping of the ZF. At small $\eta$ (blue circles and red triangles), $\gamma$ decreases monotonically with $u$. However, at larger $\eta$ (green squares), $\gamma$ increases at large $u$, which is consistent with Ref. [2] (cf. Fig. 3 therein).

[1] M. Barnes *et al.*, GS2 v8.0.2, https://doi.org/10.5281/zenodo.2645150.
[2] B. N. Rogers, W. Dorland, and M. Kotschenreuther, Phys. Rev. Lett. **85**, 5336 (2000).
[3] W. D. Dorland, Ph.D. Thesis, Princeton University (1993).
[4] I. G. Abel, M. Barnes, S. C. Cowley, W. Dorland, and A. A. Schekochihin, Phys. Plasmas **15**, 122509 (2008).
[5] M. Barnes, I. G. Abel, W. Dorland, D. R. Ernst, G. W. Hammett, P. Ricci, and T. Tatsuno, Phys. Plasmas **16**, 072107 (2009).
[6] M. N. Rosenbluth and F. Hinton, Phys. Rev. Lett. **80**, 724 (1998).
